# Supplementary material for: VO2 Nanocrystals for Designer Phase-Change Metamaterials
Source: arXiv:1911.12782 source file (2019-11-28)
Supplement: Supplementary file 1 [file Supplementary_Information_VO2-NCs_John_et_al_Final.pdf]

# Supporting Information

# $VO_2$ nanocrystals for designer phase-change metamaterials

*Jimmy John, Yael Gutierrez, Zhen Zhang, Helmut Karl, Shriram Ramanathan, Régis Orobtchouk, Fernando Moreno, and Sébastien Cueff*

## Section 1: Spectroscopic ellipsometry measurements and analysis

### Theory:

Spectroscopic ellipsometry is an optical technique used to measure the spectral amplitude (tan $\psi$) and phase ($\Delta$) of the reflected light which are related to the optical properties and microstructure of the sample under study. It is defined by:

$$\tan(\psi)\, e^{i\Delta} = R_p / R_s = [(\varepsilon)^{1/2}\cos\phi_1 - (\varepsilon_1)^{1/2}\cos\phi] / [(\varepsilon_1)^{1/2}\cos\phi - (\varepsilon)^{1/2}\cos\phi_1] \qquad (S1)$$

Where $\varepsilon_1$ is the dielectric function of the incident medium (air) and $\phi_1$ is the angle of incidence and $\phi$ the reflected light beam. The enabling principle of ellipsometry is that *p-* and *s-* polarized light reflect differently ($Rs \neq Rp$). We therefore measures the change of phase and polarization of light, which enables the determination of the sample's complex dielectric function ($\varepsilon$) [1].

### *Is*, *Ic* parameters:

In the case of phase-modulated ellipsometer, like the one we use, we do not measure $\psi$ and $\Delta$ directly. Instead, we measure functions of $\psi$ and $\Delta$. Here, we measure *Is* and *Ic* which are defined as:

$$Is = \sin(2\psi).\sin(\Delta), \qquad (S2)$$

$$Ic = \sin(2\psi).\cos(\Delta), \qquad (S3)$$

These trigonometric functions *Is* and *Ic* are directly related to $\psi$ and $\Delta$. They depend on the measurement conditions, in our case these above equations are only valid for the situation when analyzer is at 45° and the modulator at 0°. Throughout this work, we directly fit the theoretical models to the *Is* and *Ic* values.

### Data Acquisition and Optical Modeling of $VO_2$:

The complex dielectric functions of thin films of $VO_2$ and their thicknesses can be derived by fitting realistic optical models to the experimental data. The acquired ellipsometric parameters *Is* and *Ic* of the thin film sample have been collected for varying angles 55° - 75° over a spectrum range of 260 - 2100 nm.

We analyzed a 25-nm-thick $VO_2$ thin-film deposited on $SiO_2$. The acquisition was carried out in a range of temperatures from 30°C to 80°C using a digitally controlled heat cell (Linkam THMSEL350V). The substrate response was modeled using dispersion formula by Malitson et al [2].

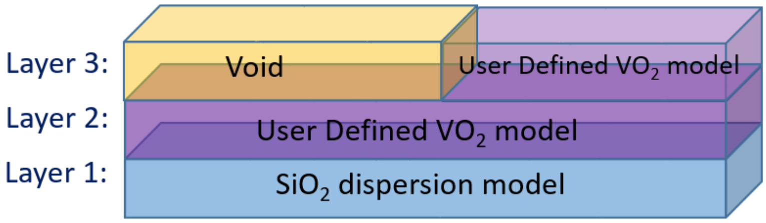


*Figure 1: Optical model: Layer by layer modelling of $VO_2$ on $SiO_2$*

To model the complex permittivity of $VO_2$ we used the Tauc-Lorentz model with three oscillators and an additional Drude model for the metallic state. Figure 1 shows the multi-layer model composed of three layers: top layer (Layer 3) being the roughness layer ($VO_2$ model + Void) which is expressed by an effective medium approximation (EMA) with Bruggeman formula [3], followed by the $VO_2$ (Layer 2) (thickness calibrated during deposition and then the substrate (Layer 1). The model is then subject to free fit using least-squares curve fitting thanks to the Levenberg-Marquardt algorithm.

## Oscillators and dispersion function for $VO_2$ model:

Commonly used dispersion functions include Cauchy and Lorentz (Classical) for transparent or weakly absorbing films, amorphous, new amorphous, and Tauc-Lorentz for semi-transparent materials (dielectrics, polymers, semiconductors absorbing in the VIS/FUV), and Drude for metals.

We model the optical properties of $VO_2$, by the sum of three Tauc-Lorentz oscillators, each of which corresponding to inter-band transitions in the material [4]. The equation that expresses the complex permittivity ($\varepsilon_1 + i\,\varepsilon_2$) using Tauc density of state and Lorentz oscillators is given below.

$$\tilde{\varepsilon}_{TL} = \varepsilon_{r,TL} + i.\varepsilon_{i,TL} = \varepsilon_{r,TL} + i.\varepsilon_{i,T} \times \varepsilon_{i,L}) \qquad \text{(S4)}$$

The imaginary part of Tauc's dielectric function describes inter-band transitions above the band edge and Lorentz part describes inter-band transitions as dielectric oscillators. The combination of both is expressed by the equation below.

$$\varepsilon_i = \begin{cases} \sum_{i=1}^{N} (\frac{1}{E}) \times \frac{A_i.E_i.C_i.(E-E_g)^2}{(E^2-E_i^2)^2+C_i^2.E^2}, & E > E_g \\ 0, & E \leq E_g \end{cases} \qquad \text{(S5)}$$

Where $A_i$ is the strength of $\varepsilon_{i,\,TL}\,(E)$ peak, $C_i$ represents the broadening of the peak and $E_i$ is the peak energy, where *'i'* corresponds to oscillator values. The corresponding real part of their dielectric functions, as shown below, is derived from the expression, $\varepsilon_i$ using Kramers-Kronig integration:

$$\varepsilon_r(E) = \varepsilon_r(\infty) + \sum_{i=1}^{N} (\frac{2}{\pi}).P.\int_{-\infty}^{\infty} \frac{\varepsilon_i(\xi).\xi}{\xi^2 - E^2} \qquad \text{(S6)}$$

where *P* denotes Cauchy's principal values.

The Drude contribution for the behavior of $VO_2$ at its metallic state is given by:

$$\varepsilon = \frac{\omega_p^2}{-\omega^2 + i\Gamma_D\omega} \qquad \text{(S7)}$$

Where, $\omega_p$ is the plasma frequency, $\omega$ is the frequency of the incident electromagnetic field and $\Gamma_D$ (in eV) is the collision frequency (damping factor), which increases the broadening of absorption tail. The damping effect is due to the absorption and collision processes of free carriers.

The initial parameters for the fitting calculations and the number of oscillators to be used were set on the basis of previous reports about the determination of dielectric spectra of $VO_2$ [4].

Such a model is physically consistent and, as detailed below, each variable parameter represents a physical quantity:

- $\boldsymbol{\varepsilon_r\,(\infty) = \varepsilon_\infty}$ is the high frequency dielectric constant. This fitting parameter prevents $\varepsilon_1$ from converging to zero for energies below the band gap and it is generally, $\varepsilon_\infty > 1$.
- $\boldsymbol{A_i}$ (in eV) is related to the strength of the $i^{th}$ absorption peak. The subscript *'i'* refers to the number (i =1, 2 or 3) of oscillators. As $A_i$ increases, the amplitude of the peak increases and the Full Width at Half Maximum (FWHM) of that peak gets slightly larger.
- $\boldsymbol{C_i}$ (in eV) is the broadening term; it is a damping coefficient linked to the FWHM of the $i^{th}$ peak of absorption. The higher it is, the larger the peak becomes and at the same time the smaller its amplitude.
- $\boldsymbol{E_g}$ (in eV) is the optical band gap energy.

- $\boldsymbol{E_i}$ (in eV) is the energy of maximum transition probability or the energy position of the peak of absorption. The subscript '*i*' refers to the number (i =1, 2 or 3) of oscillators. Always, $E_g < E_i$.

As displayed in figure 2, we obtain a very good agreement between the experimentally measured ellipsometric parameters *Is/Ic* and the simulated optical model described above, with $\chi^2 = 0.59$.

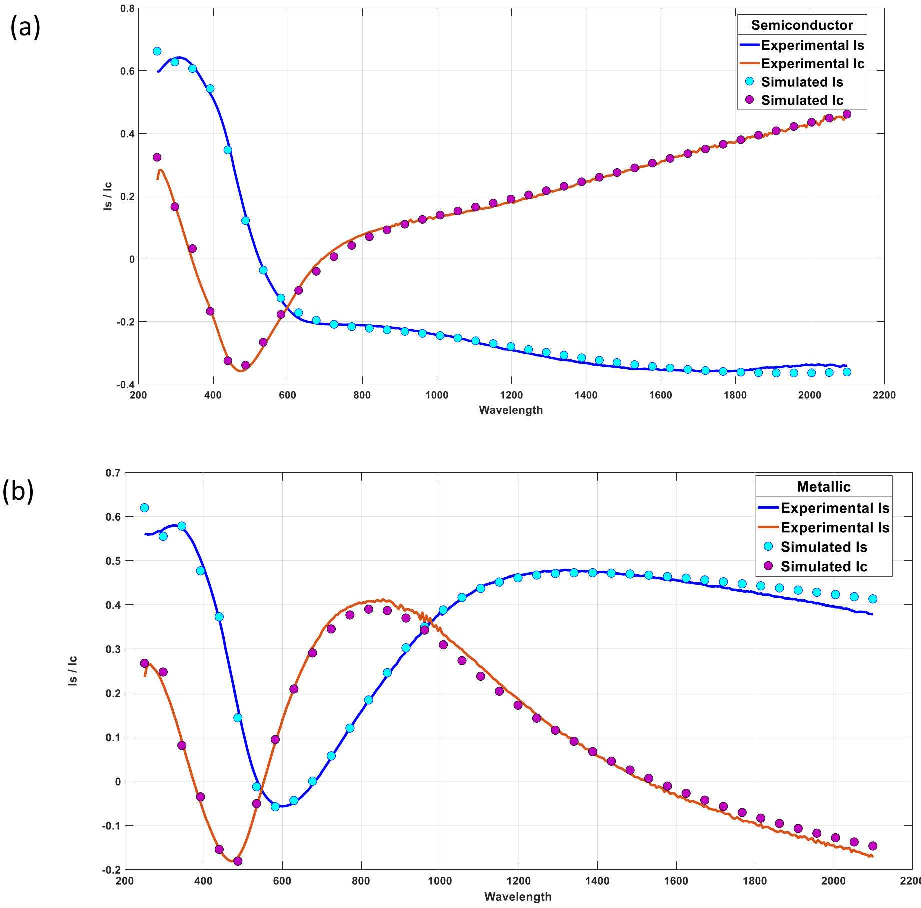


*Figure 2: Fitting the optical model and experimental data. (a) Experimental and simulated Is/Ic parameters for semiconductor state of $VO_2$ (b) Experimental and simulated Is/Ic parameters for metallic state.*

Figure 3 shows the optical dispersion of $VO_2$, extracted from the fits to the experimental data in both states of $VO_2$. The corresponding values obtained for the variable fit parameters are given in Table 1.

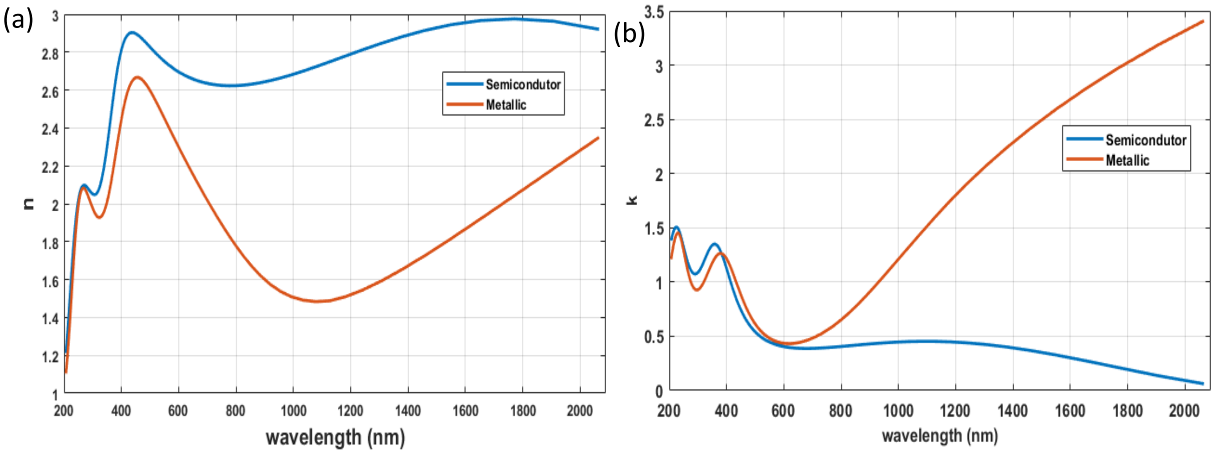


*Figure 3: Optical dispersion of $VO_2$ as extracted from the fits (a) refractive index (n). (b) Extinction coefficient (k).*

| $VO_2$ state 1: Semiconductor | | $VO_2$ state 2: Metallic | |
|---|---|---|---|
| Fit Parameters | Values | Fit Parameters | Values |
| ε∞ | 1.944 | ε∞ | 1.421 |
| Eg | 0,535 | Eg | 0,06 |
| 3 x Tauc-Lorentz Oscillator Values | | | |
| $A_1$ | 13.48 | $A_1$ | 14.63 |
| $E_1$ | 3.53 | $E_1$ | 3.069 |
| $C_1$ | 1.477 | $C_1$ | 1.662 |
| $A_2$ | 15.89 | $A_2$ | 44.51 |
| $E_2$ | 5.85 | $E_2$ | 6.02 |
| $C_2$ | 2.57 | $C_2$ | 5.10 |
| $A_3$ | 29.58 | $A_3$ | 1.646 |
| $E_3$ | 0.49 | $E_3$ | 0.46 |
| $C_3$ | 1.05 | $C_3$ | 3.10 |
| Drude values | | | |
| ω | - - | ω | 3.872 |
| г | - - | г | 0.654 |

*Table 1: Fit parameter values obtained for both the states of $VO_2$.*

## Experimental ellipsometry parameters used to measure $VO_2$-NCs:

We have first characterized the real-time dynamics of the insulator-to-metal transition of $VO_2$-NCs using the kinetic mode of our ellipsometer.

In the kinetic mode, ellipsometric data are acquired every 200 ms at a fixed wavelength (in this case 1200 nm). Here, the kinetic data are shown (Figure 4a) during the evolution of phase change $VO_2$ NCs by actively mapping the change in dielectric function (denote by the component *Ic*). The heat cell is automatized to gradually increase the temperature at a given rate 1°C/min, the acquisition ranged from 23°C (room temperature) to 150°C.

The hysteretic behavior as a function of temperature is shown in Fig. 4b, where the difference between the heating (red) and cooling (blue) cycles are put into evidence. The hysteresis loop is large, (differences in switching temperatures between heating and cooling ~35°C), as expected from $VO_2$-NCs.

Through kinetic probing and hysteresis measurements we observed a good optical modulation, typical from the $VO_2$ IMT. But in comparison with the bulk we observe a shift in transition temperature for NCs, as its initiation occurs later than that of bulk.

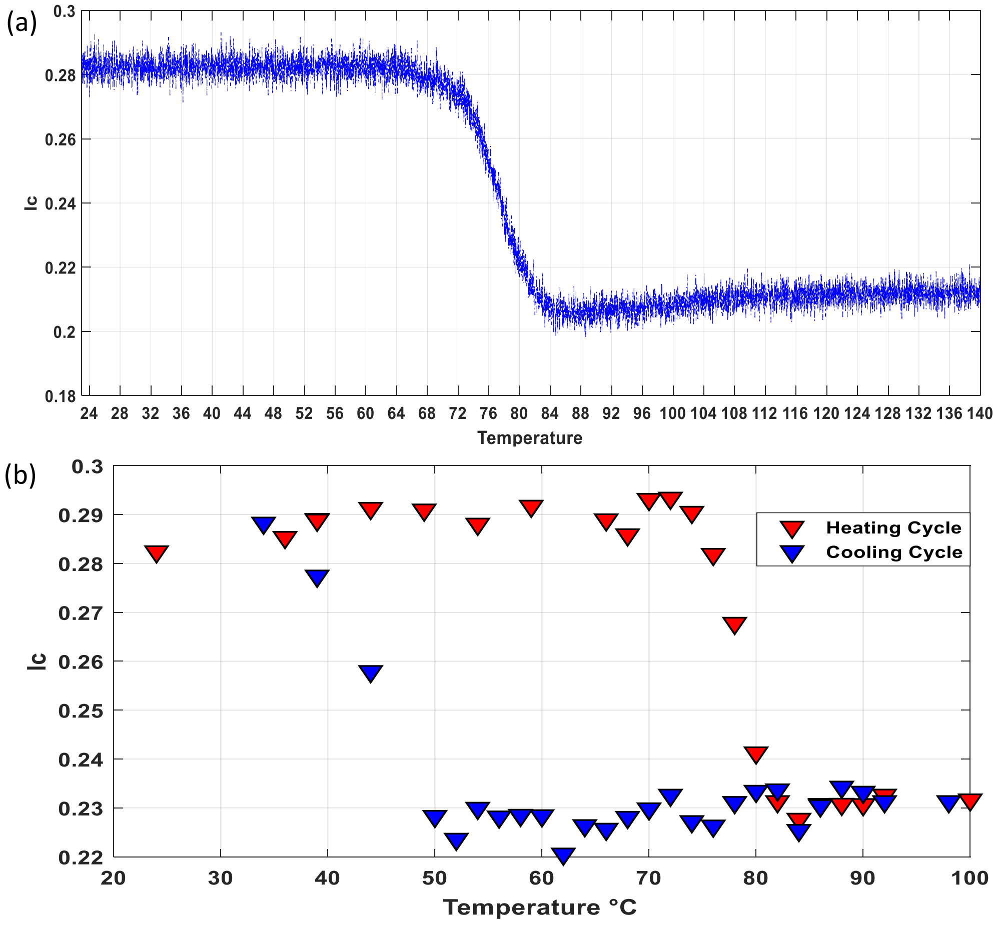


*Figure 4 (a): Dynamic optical measurements of the $VO_2$ NCs IMT. (b): Thermal Hysteresis loop of $VO_2$ NCs.*

As similarly done previously for the $VO_2$ thin-films, we create an optical model for $VO_2$ NC. The model description of the sample is showed in Figure 5.

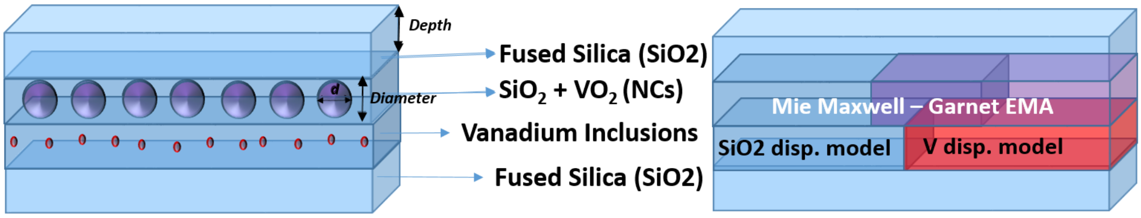


*Figure 5: 3D representation of optical stacks for $VO_2$ NC embedded in fused silica.*

Figure 5 shows a multi-layer model composed of four layers: the top layer is $SiO_2$ (fused silica), followed by optical models of $VO_2$-NC, whose value were computed using the Mie-Maxwell-Garnet effective medium (more details on the model in the main text). Following previous TEM analysis, we know that during the implantation of nanocrystals, some of the implanted $V^+$ ions have penetrated at further depth, therefore an intermediate layer containing vanadium inclusions is added as an EMA of Vanadium metal and $SiO_2$ followed by the substrate. The value associated with the thickness and the depth of the embedded $VO_2$ NC is used as a free fit parameter and is consistent with the experimental implantation data.

## Section 2: Derivation of the expressions for effective permittivity and permeability

The effective dielectric constant $\overline{\epsilon}$ of a suspension of small spherical particles of radius $a$ embedded in a host medium of dielectric constant $\epsilon_h$ is given by the Clausius–Mossotti equation

$$\frac{\overline{\epsilon}-\epsilon_h}{\overline{\epsilon}+2\epsilon_h} = \frac{f}{a^3}\alpha \quad (1)$$

Where $\alpha$ is the particle dipolar polarizability and $f$ is the volume fraction of the embedded particles. Under the electrostatic approximation, the particle dipolar polarizability can be written as

$$\alpha = \frac{\epsilon_i-\epsilon_h}{\epsilon_i+2\epsilon_h} a^3 \quad (2)$$

Where $\epsilon_i$ is the dielectric constant of the sphere material. When (2) is substituted in (1) one obtains the usual Maxwell Garnett formula.

$$\frac{\overline{\epsilon}-\epsilon_h}{\overline{\epsilon}+2\epsilon_h} = f\frac{\epsilon_i-\epsilon_h}{\epsilon_i+2\epsilon_h} \quad (3)$$

This equation, which is independent of the sphere radius $a$, is only valid for sphere sizes much smaller than the illuminating wavelength $\lambda$. To overcome this problem, the electric dipole polarizability can be written in terms of the Mie coefficient $a_1$ by [5]

$$\alpha_E = \frac{i3a^3}{2x^3} a_1 \quad (4)$$

where the size parameter $x$ is defined as

$$x = \frac{2\pi a\sqrt{\epsilon_h}}{\lambda} \quad (5)$$

By introducing (4) in (1) it is possible to obtain the expression for the effective dielectric function used in the main text (eq. (4)) [6,7],

$$\overline{\epsilon} = \frac{x^3+3ifa_1}{x^3-\frac{3}{2}ifa_1} \quad (6)$$

Symmetrically, and attending to the dipolar magnetic Mie coefficient $b_1$, is it possible to define a magnetic dipole polarizability as [5]:

$$\alpha_H = \frac{i3a^3}{2x^3} b_1 \quad (7)$$

Therefore, in analogy with the derivation of (6), the expression for an effective magnetic permeability $\overline{\mu}$ is given by [6,7]

$$\overline{\mu} = \frac{x^3+3ifb_1}{x^3-\frac{3}{2}ifb_1} \quad (8)$$

## Section 3: Modelling the effect of interactions between nanoparticles

The Mie theory-based extension of Maxwell-Garnett effective medium approximation, i.e., approach used to predict the optical behavior of slab composed by $VO_2$ nanospheres embedded in quartz (see eqs. 4-5 in the main text), does not take into account the possible interaction between nanocrystals (NCs). In principle, given the mean separation of the NCs [8], interaction effects are expected to be small. However, to have a better estimation of how interaction effects may affect the plasmonic response of the NCs, we have calculated the absorption cross-section ($C_{abs}$) of dimers made of insulating and metallic $VO_2$ spherical NPs for different inter-particle distances (gaps) embedded in quartz. The spheres have a size of 70 nm (as the spheres used for the calculations of the effective optical properties (see Figure 4 in main text)) and the considered gaps range between 10 and 150 nm. These calculations have been performed for three polarizations (Fig. 6): x-polarization (i.e. along the dimer axis), y-polarization (i.e. perpendicular to the dimer axis) and at 45° (This angle is chosen because the incident polarization used in the ellipsometry experiments is linear at 45° with the incidence plane).

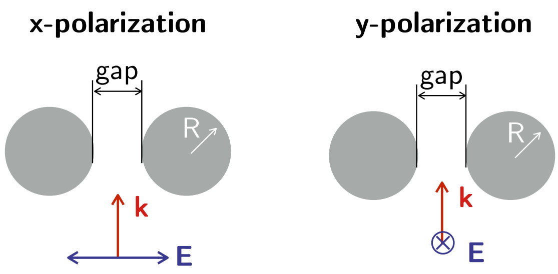


*Figure 6. Scheme of the two analyzed systems: dimer formed by spheres (R = 25 nm) separated by a gap and illuminated with x- (left) and y-polarized beams (right). With arrows are represented the polarization of the illuminating beam (**E**, blue arrow) and the wave vector (**k**, red arrow).*

Calculations have been performed using commercial software FDTD solutions Version 8.16 from Lumerical Inc. Total field/scattered field light source conditions were used in all simulations. An illuminating linearly polarized plane-wave was set to propagate perpendicular to the dimer axis. The wavelength spectral range analyzed was from 260 to 1500 nm to mimic experimental conditions. A non-uniform mesh was used in the simulation region. A finer mesh was defined in the vicinity of the NPs. In this region, the mesh step was fixed to $d_x = d_y = d_z = 2$ nm. The absorption cross-section was calculated within the total-field/scattered-field formalism.

### $VO_2$ dimers in its metallic phase

Figure 7 shows how the Localized Surface Plasmon Resonance (LSPR) peaks appearing in the absorption cross-section ($C_{abs}$) of a dimer made of metallic $VO_2$ nanospheres are affected by the interparticle distance (gap). With dashed black lines are represented the peak positions for a system of two non-interacting spheres (the two most left lines correspond to the electric and magnetic dipole resonances, respectively). In this particular case we pay attention to the LSPR peak appearing at 1176 nm which has a pure dipolar electric character. Figure 7(a) shows how, for the dimer illuminated with x-polarized light, the LSPR peak is red-shifted as the gap becomes smaller, reaching a maximum shift of 110 nm for a gap of 5 nm. On the contrary, Figure 7(b) shows that the LSPR peak is blue-shifted when the dimer is illuminated with an y-polarized beam. The maximum blue-shift is 30 nm for a gap of 10 nm. These results are consistent with those reported by Rechberger *et al.* [9].

Because the samples under study are randomly distributed inside the quartz slide, we can consider that, on average, the effect of the interaction has an intermediate effect between the two extreme situations:

x-polarization and y-polarization. Consequently, Figure 7(c) shows how the absorption cross-section of the dimer is affected for different gaps when it is illuminated with 45° linearly polarized light. As the gap decreases, the LSPR peak is redshifted. The maximum shift is 40 nm approximately and it is produced for the smallest gap.

These results support the idea that the electromagnetic interaction between $VO_2$-NCs are causing the discrepancy between the fitting and the experimental measurements in Figure 4(b).

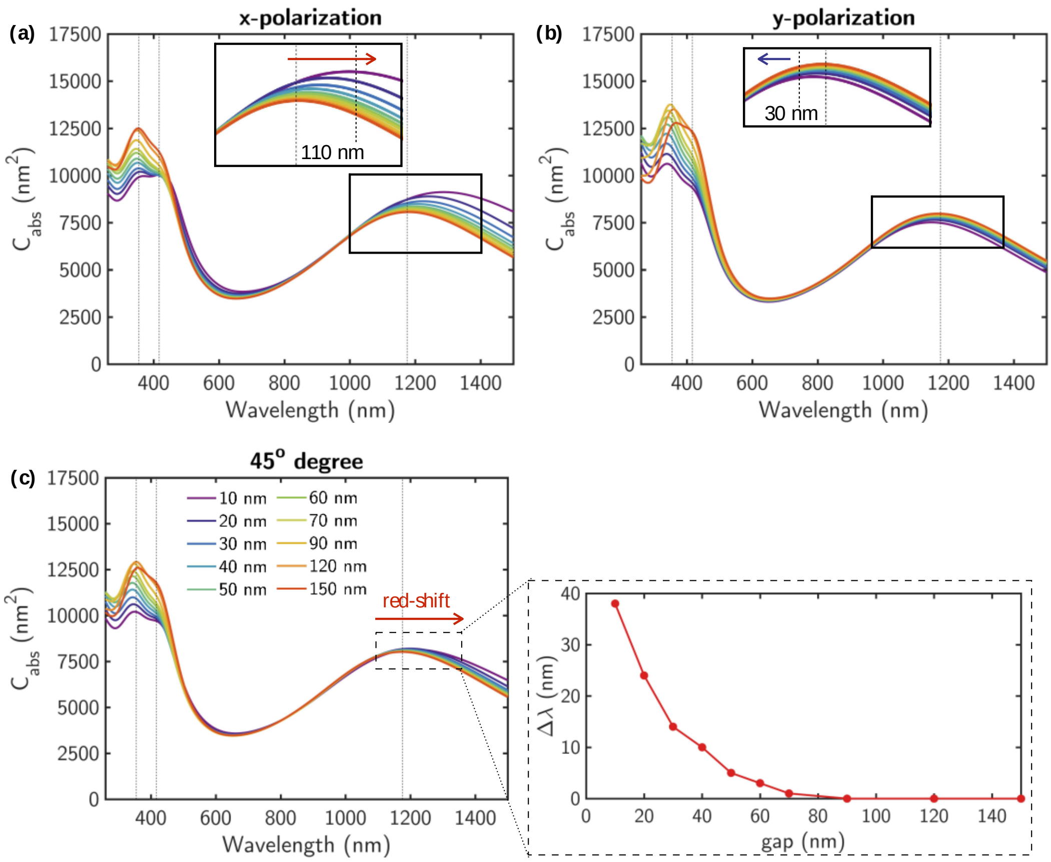


*Figure 7. Absorption cross-section ($C_{abs}$) of $VO_2$ dimers in its metallic phase (R = 35 nm) when illuminated with (a) x-, (b) y- and (c) 45 °polarizations (see Fig. S1) for different interparticle distances (gaps). As an inset in (a) and (b) is indicated the maximum spectral shift between the interacting and non-interacting (dashed black lines) dimer. In (c) the spectral shift $\Delta\lambda$ is represented as a function of the gap.*

## $VO_2$ dimers in its insulating phase

Figure 8 shows how the resonance peaks appearing in the absorption cross-section ($C_{abs}$) of a dimer made of $VO_2$ nanospheres in its insulating phase are affected by its electromagnetic interaction. Again, dashed black lines represent the spectral peak positions for a system of two non-interacting spheres (as in the previous case, they correspond to a coherent mixture of dipole resonances, mainly of both electric and magnetic character). In this particular case, we pay attention to the resonance peak appearing at 381 nm whose origin is the superposition of a dipolar electric and a dipolar magnetic resonance. We study this resonance in the insulating phase in order to remove any parasitic effect coming from the dipolar electric resonance appearing at longer wavelengths in the metallic phase.

Figure 8 shows how the resonance peak is shifted with decreasing the interparticle gap for (a) x-, (b) y- and (c) 45° polarizations, respectively. For the three studied polarizations the overall effect is the same. For the largest gap (150 nm), the resonance is slightly blueshifted with respect to the non-interacting

system. With decreasing interparticle distances the resonance peak further blueshifts reaching a maximum spectral shift for an intermediate gap of 60 nm approximately. For smaller gaps the resonance peak comes back to the starting point. In this case, the resonance has two dipole contributions, one electric and one magnetic. The dimer electromagnetic interaction shifts the electric to the red part of the spectrum whilst the magnetic one is blue shifted [10]. In this case, the blue shift dominates for intermediate gap distances (60-100nm) whilst for strong interaction (gaps smaller than 50nm) the dipole electric resonance redshift compensates that of the magnetic one to the blue.

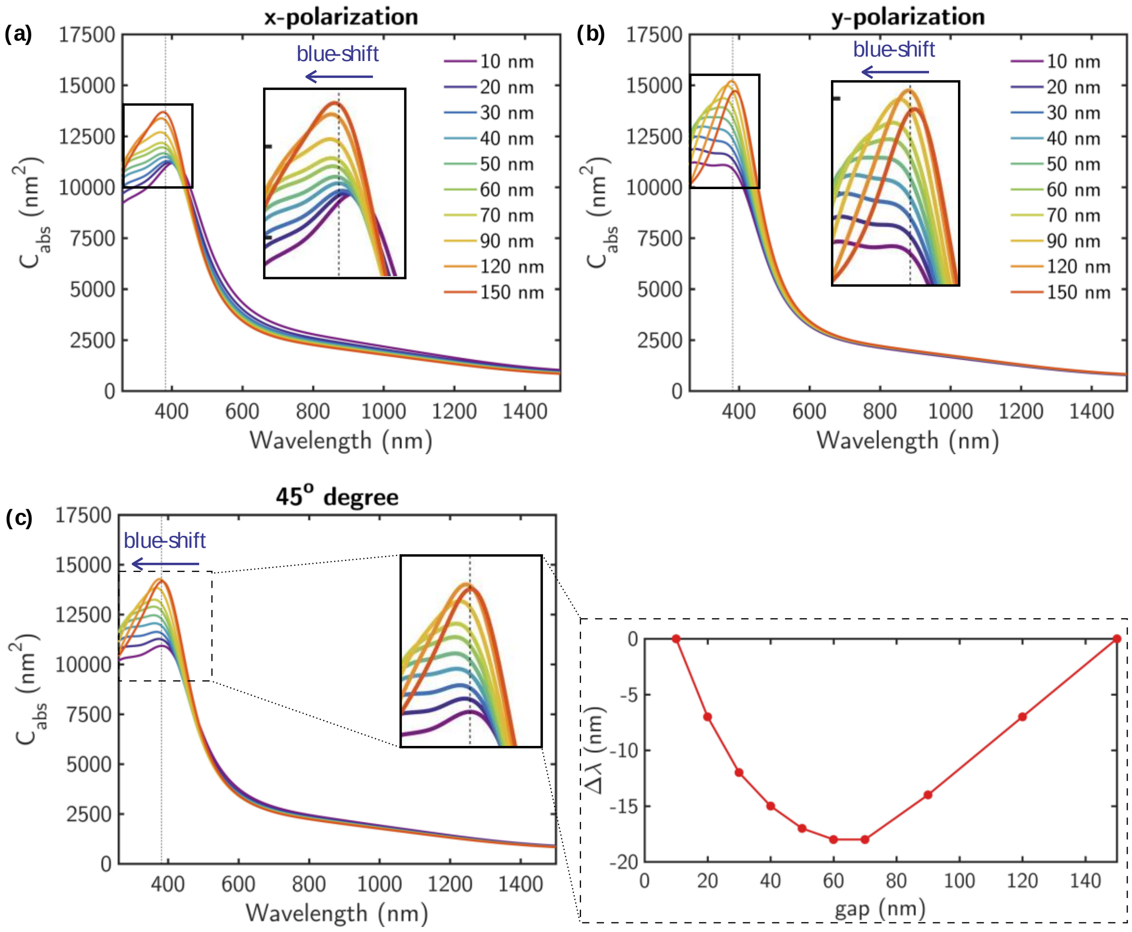


*Figure 8. Absorption cross-section ($C_{abs}$) of insulating $VO_2$ dimers (R = 35 nm) when illuminated with (a) x-, (b) y- and (c) 45 ° polarizations for different interparticle distances (gaps). As an inset in (a) and (b) is indicated the maximum spectral shift between the interacting and non-interacting (dashed black lines) dimer. In (c) the spectral shift $\Delta\lambda$ is represented as a function of the gap.*

## Section 4: Modelling the polydispersity in size distribution of nanoparticles

In the approach used to predict the optical behavior of a slab composed by $VO_2$ nanospheres embedded in quartz (Mie theory-based extension of Maxwell-Garnett effective medium approximation) the effect of the potential polydispersity of the NCs in the sample is not included. All the calculations assume that all NCs have the same size (in our case their radius R is assumed to be 35 nm and is taken as the reference system). However, some polydispersity is expected. In order to evaluate the effect that this phenomenon may have on the spectral resonances, Fig. 9 shows the difference in the absorption cross-section spectra ($C_{abs}$) between the reference system (R = 35 nm) and two other systems with a well-defined polydispersities. The first has a symmetric size distribution centered around the reference size. The other system has an asymmetric size distribution, having a majority of NCs with the reference size, but others with larger sizes. For this study we will focus on the resonance (LPSR) appearing at ≈ 1176 nm in the $VO_2$ NCs in their metallic phase.

As an example, Fig. 9(a) shows the $C_{abs}$ spectra for the reference system and the one with the symmetric NCs size distribution (Fig. 9(b)). In this case, there is no significant difference between both systems. On the contrary, in the case of the asymmetric NCs size distribution (Fig. 9(c)) there are significant differences. The LSPR appearing in the $C_{abs}$ spectrum of the polydisperse sample, as shown in Fig. 9(c), is redshifted (20 nm) and also broader than the reference system.

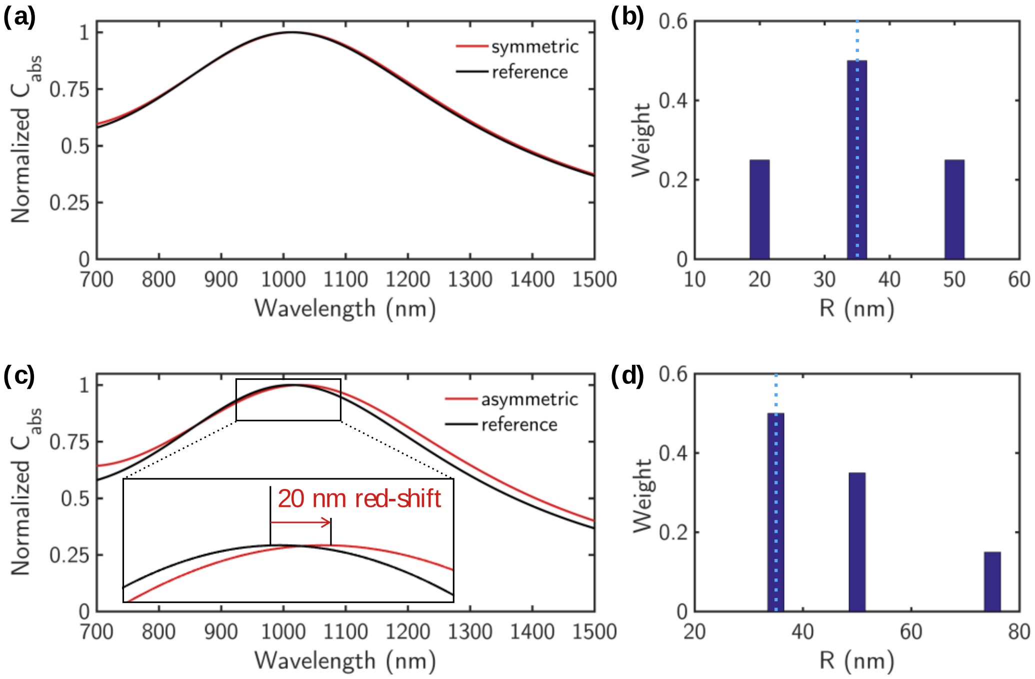


*Figure 9. Absorption cross-section ($C_{abs}$) spectra for the reference monodisperse system (R = 35 nm, black line) and others with (a) symmetric and (c) asymmetric distribution of NC sizes. Size distribution of the (b) symmetric and (d) asymmetric systems. With the light dotted line is represented the size of the monodisperse distribution.*

## References:


[1]. H. G. Tompkins, and E. A. Irene, Handbook of ellipsometry (William Andrew, New York, 2005).

[2]. I. H. Malitson. Interspecimen comparison of the refractive index of fused silica, J. Opt. Soc. Am. 55, 1205-1208 (1965)

[3]. Fujiwara, H., Koh, J., Rovira, P., Collins, R. Assessment of effective-medium theories in the analysis of nucleation and microscopic surface roughness evolution for semiconductor thin films (2000) 61 (16), pp. 10832-10844. DOI: 10.1103/PhysRevB.61.10832.

[4]. Gavini, A., Kwan, C.C.Y. 22975240400; 22976230700; Optical properties of semiconducting $VO_2$ films, DOI: 10.1103/PhysRevB.5.3138

[5]. Mulholland, G.W.; Bohren, C.F.; Fuller, K. a Light Scattering by Agglomerates: Coupled Electric and Magnetic Dipole Method. Langmuir 1994, 10, 2533–2546.

[6]. Ruppin, R. Evaluation of extended Maxwell-Garnett theories. Opt. Commun. 2000, 182, 273–279.

[7]. Doyle, W.T. Optical properties of a suspension of metal spheres. Phys. Rev. B 1989, 39, 9852–9858.

[8]. M.I. Mishchenko, L.D. Travis, Polarization and Depolarization of Light, in Light Scattering from Microstructures., F. Moreno and F. González Eds. (Springer-Verlag, 2000) doi:10.1007/3-540-46614-2

[9]. Rechberger, W. et al. Optical properties of two interacting gold nanoparticles. Opt. Commun. 220, 137–141 (2003).

[10]. Albella, P. et al. Low-Loss Electric and Magnetic Field-Enhanced Spectroscopy with Subwavelength Silicon Dimers. J. Phys. Chem. C 117, 13573−13584 (2013)


.

.
